# Supplementary material for: Dark Energy Survey Year 3 Results: Clustering Redshifts -- Calibration of the Weak Lensing Source Redshift Distributions with redMaGiC and BOSS/eBOSS
Source: arXiv:2012.08569 source file (2020-12-15)
Supplement: Supplementary file 1 [file Appendix.tex]

\section{Transferring the WL selection function from the wide field to a small deep field}\label{sect:AppendixA}

We describe here how we apply a given sample selection as measured in a wide field to a smaller (but  deeper) field. In the DES Y3 case,  this is used to apply the WL selection function (which   depends on both galaxy properties and observing conditions as measured across the Y3 footprint) to the deep fields, where a small, deep sample with very good redshift is available. Once such a selection is applied to the deep field, one can directly use the deep field to estimate the WL galaxy bias evolution.

To achieve this, we make use of a transfer function. Let us denominate the  measured properties  of  a galaxy observed in the wide field with $\bf{\hat{x}}$, and those of  a galaxy observed in the deep field with $\bf{x}$. These properties can be observed fluxes, magnitudes, etc. Let us assume that with some clustering methods we can assign galaxies to a unique cell: respectively $\bf{\hat{c}}$ in the wide field and $\bf{c}$ in the deep field. We can define define the transfer function $p(c|\hat{c},\hat{s})$, where $\hat{s}$ would be the selection function of a given sample ( in our case, the WL selection). Operationally, the transfer function is estimated from galaxies for which both deep and (possibly simulated) wide observations are available as follows:

\begin{equation}
p(c|\hat{c},\hat{s}) = \frac{\sum_{i\in\hat{s}}\delta_{c,c_i}\delta_{\hat{c},\hat{c}_i}}{\sum_{i\in\hat{s}}\delta_{c,c_i}},
\end{equation}

where $c_i$, $\hat{c}_i$ are the assigned deep and wide cells to the $i$th galaxy. We can therefore define weights for every single galaxy in the deep field so as they were affected by the same WL selection function applied in the wide field:

\begin{equation}
w_i = \sum_{\hat{c}}p(c|\hat{c},\hat{s}) p(\hat{c}|\hat{s}),
\end{equation}

with $p(\hat{c}|\hat{s})$ the fractional assignment of galaxies to cell $\hat{c}$. If a tomographic selection $\hat{B}$ is present, the weights become:

\begin{equation}
w_i = \sum_{\hat{c}\in \hat{B}}p(c|\hat{c},\hat{s}) p(\hat{c}|\hat{s}),
\end{equation}
\label{AppendixA}
