# Supplementary material for: Dark Energy Survey Year 3 Results: Clustering Redshifts -- Calibration of the Weak Lensing Source Redshift Distributions with redMaGiC and BOSS/eBOSS
Source: arXiv:2012.08569 source file (2020-12-15)
Supplement: Supplementary file 2 [file Appendix_mean_match.tex]

%\chapter[]{}
\section{Individual mean-matching likelihoods}\label{sect:Appendix_mean}

\begin{figure*}
\begin{center}
\includegraphics[width=0.9 \textwidth]{./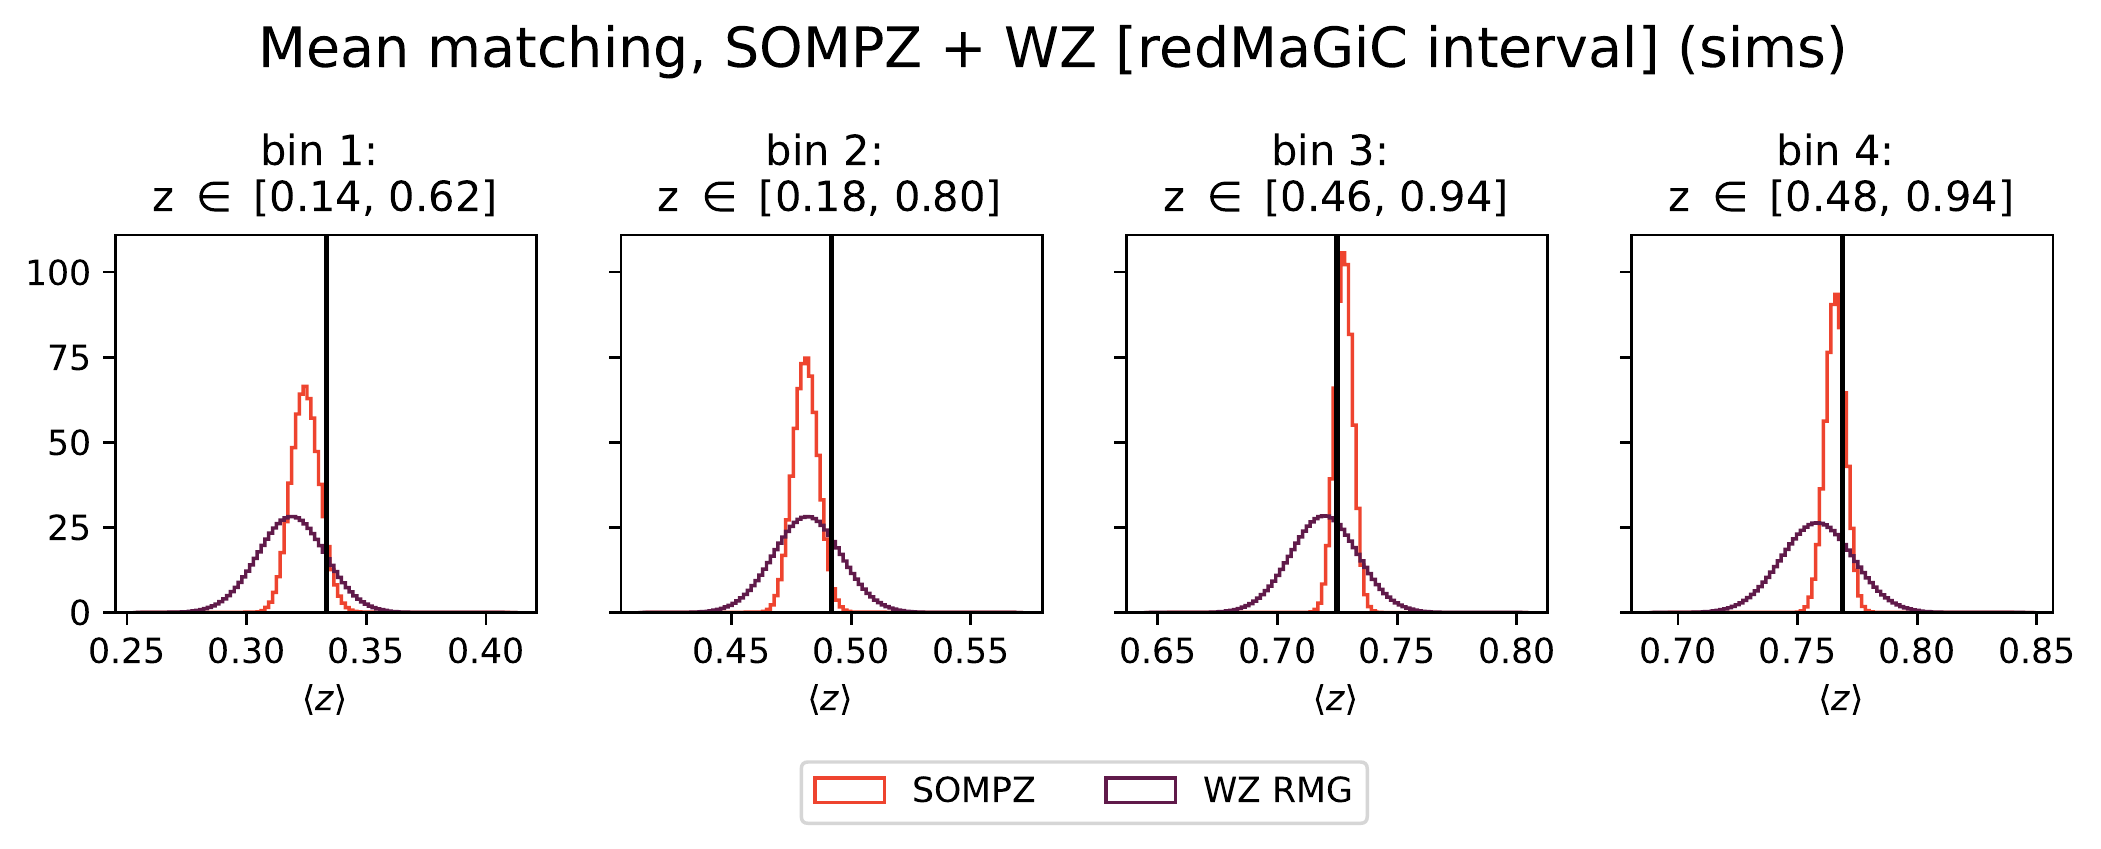}
\includegraphics[width=0.9 \textwidth]{./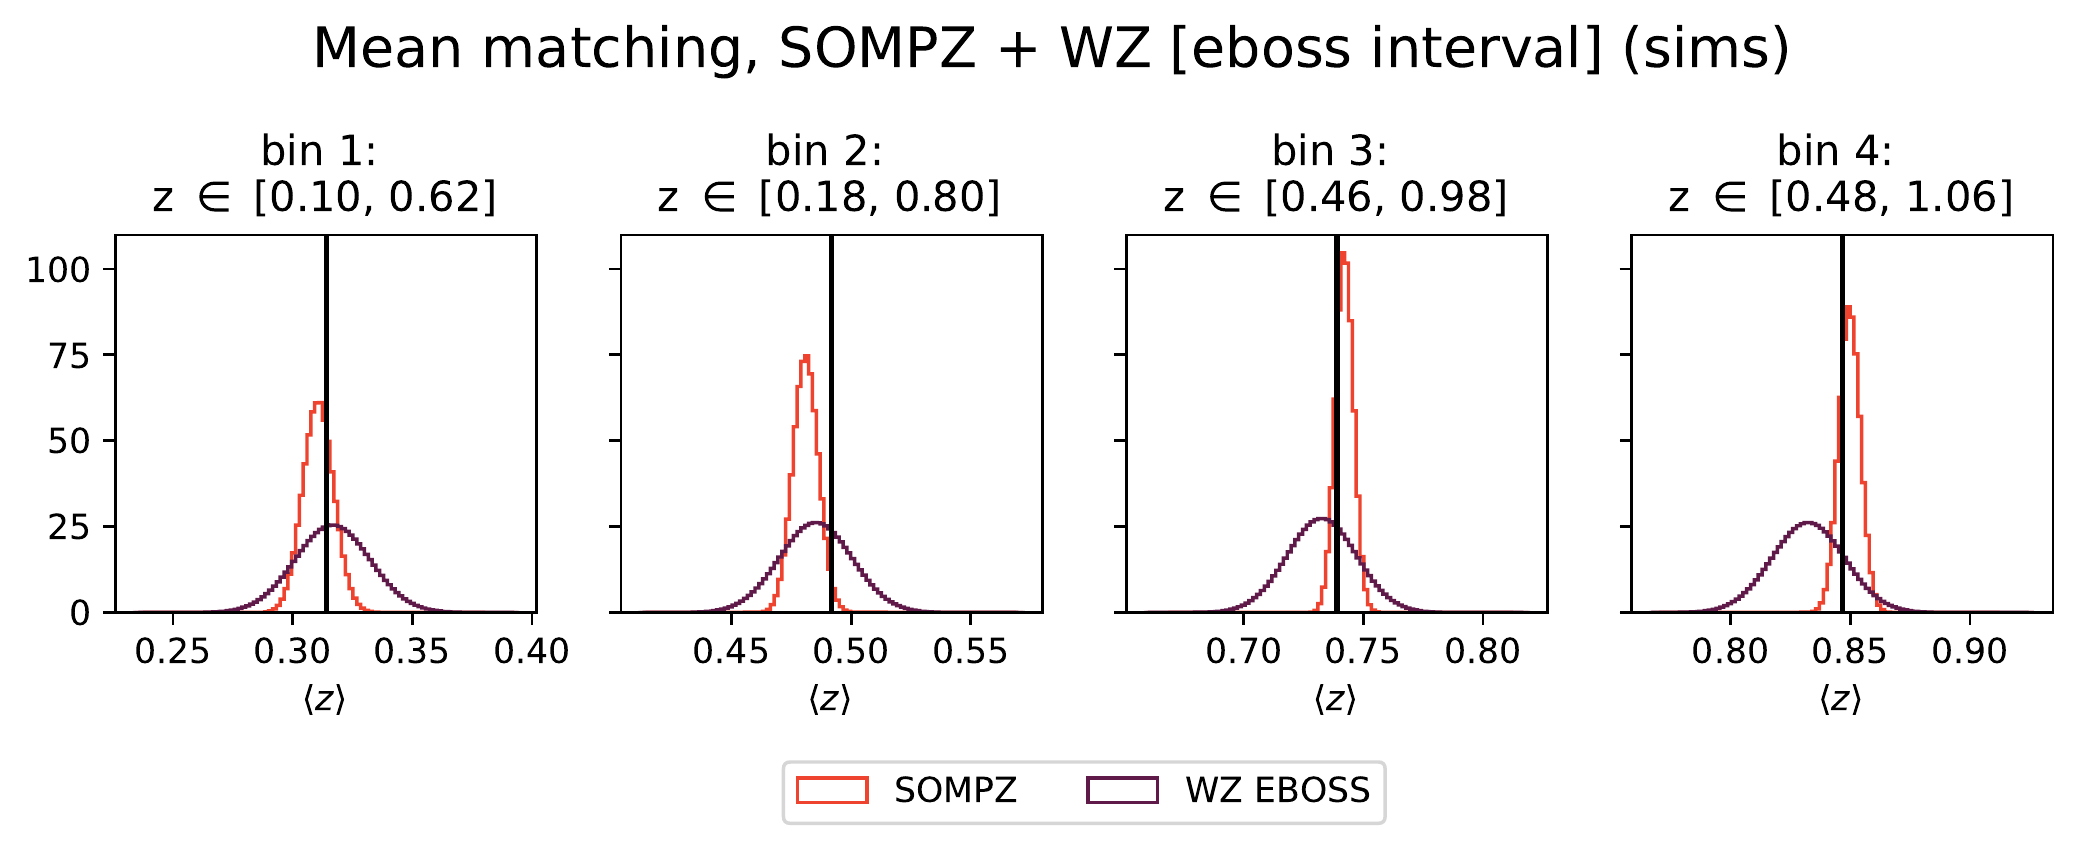}
\end{center}
\caption{Mean redshift posteriors for the 4 tomographic bins obtained using the mean matching method. The top panels show the results obtained using the \redmagic\ sample only, the lower panels show the results obtained using the BOSS/eBOSS sample only. Red histograms represent the distribution of the mean redshift of the SOMPZ realisations, while the purple histograms represent the clusttering only prior. Light-blue histograms show the mean redshift posteriors of the SOMPZ realisations using the clustering likelihood. To facilitate the comparison with the clustering prior, the mean redshift has been computed in the fiducial 2-$\sigma$ interval, i.e., excluding the tails of the redshift distributions. The black vertical lines represent the true mean redshift as computed in simulations.} 
\label{fig:dz_meanmatching_SOMPZ_WZ_individual_sims}
\end{figure*}

\begin{figure*}
\begin{center}
\includegraphics[width=0.9 \textwidth]{./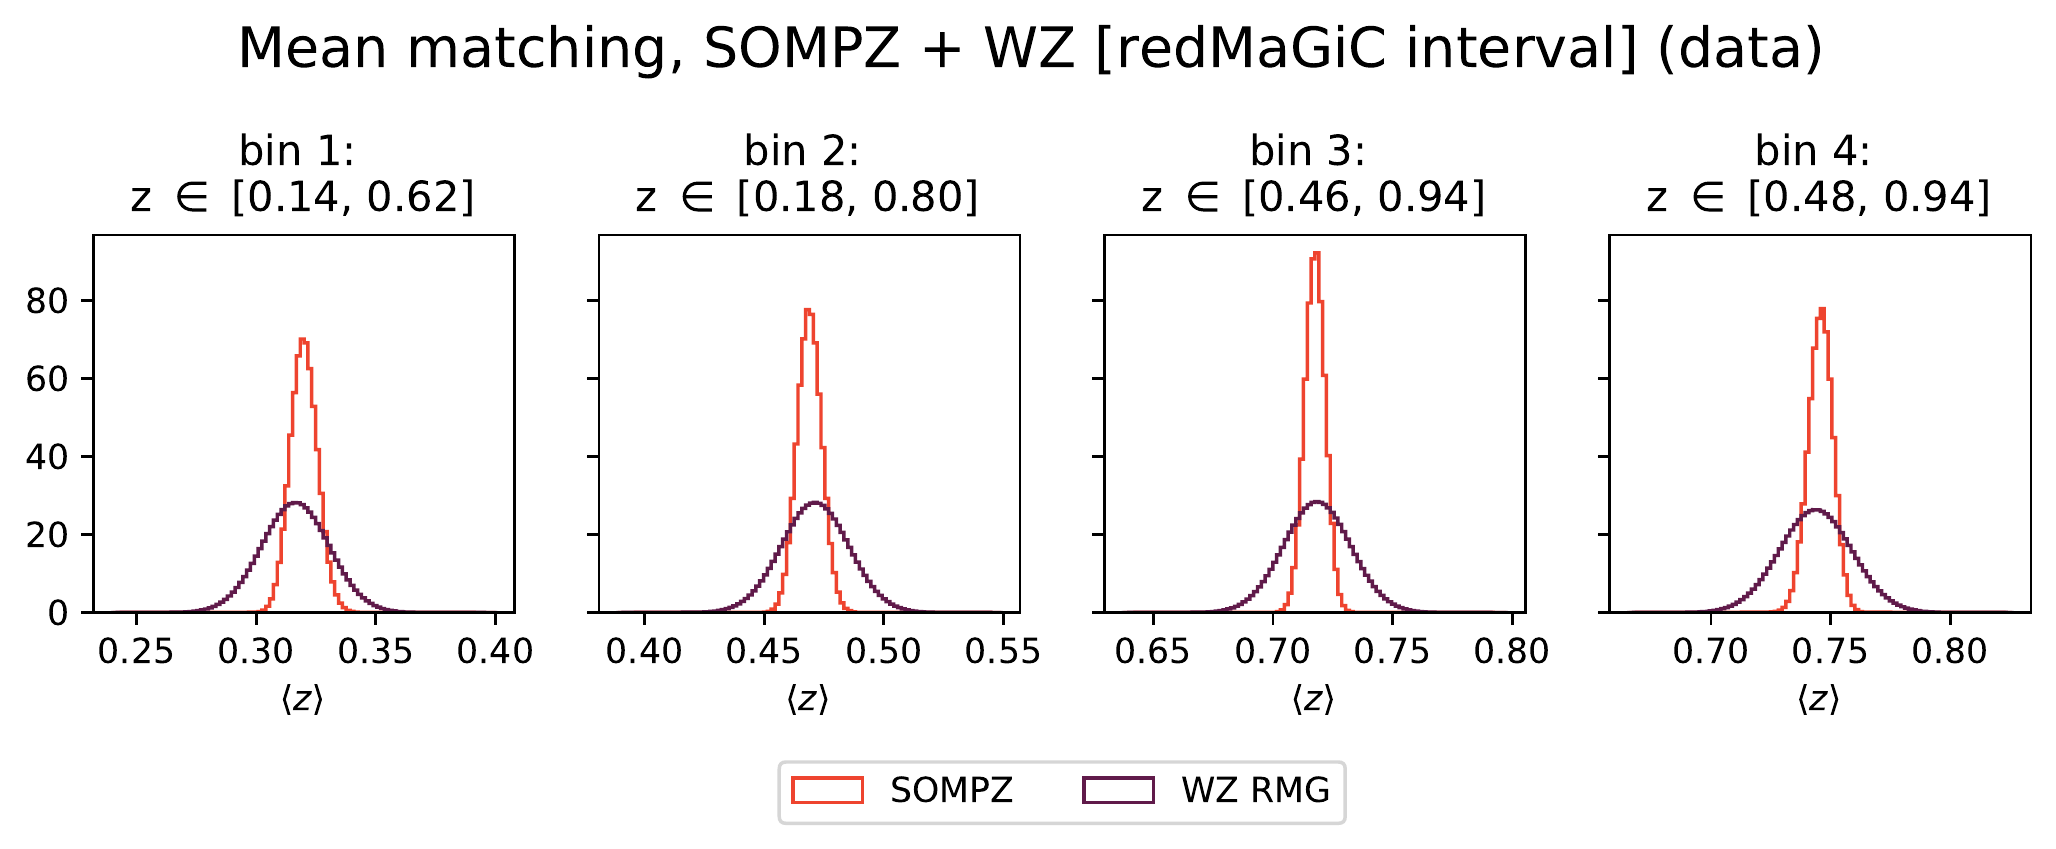}
\includegraphics[width=0.9 \textwidth]{./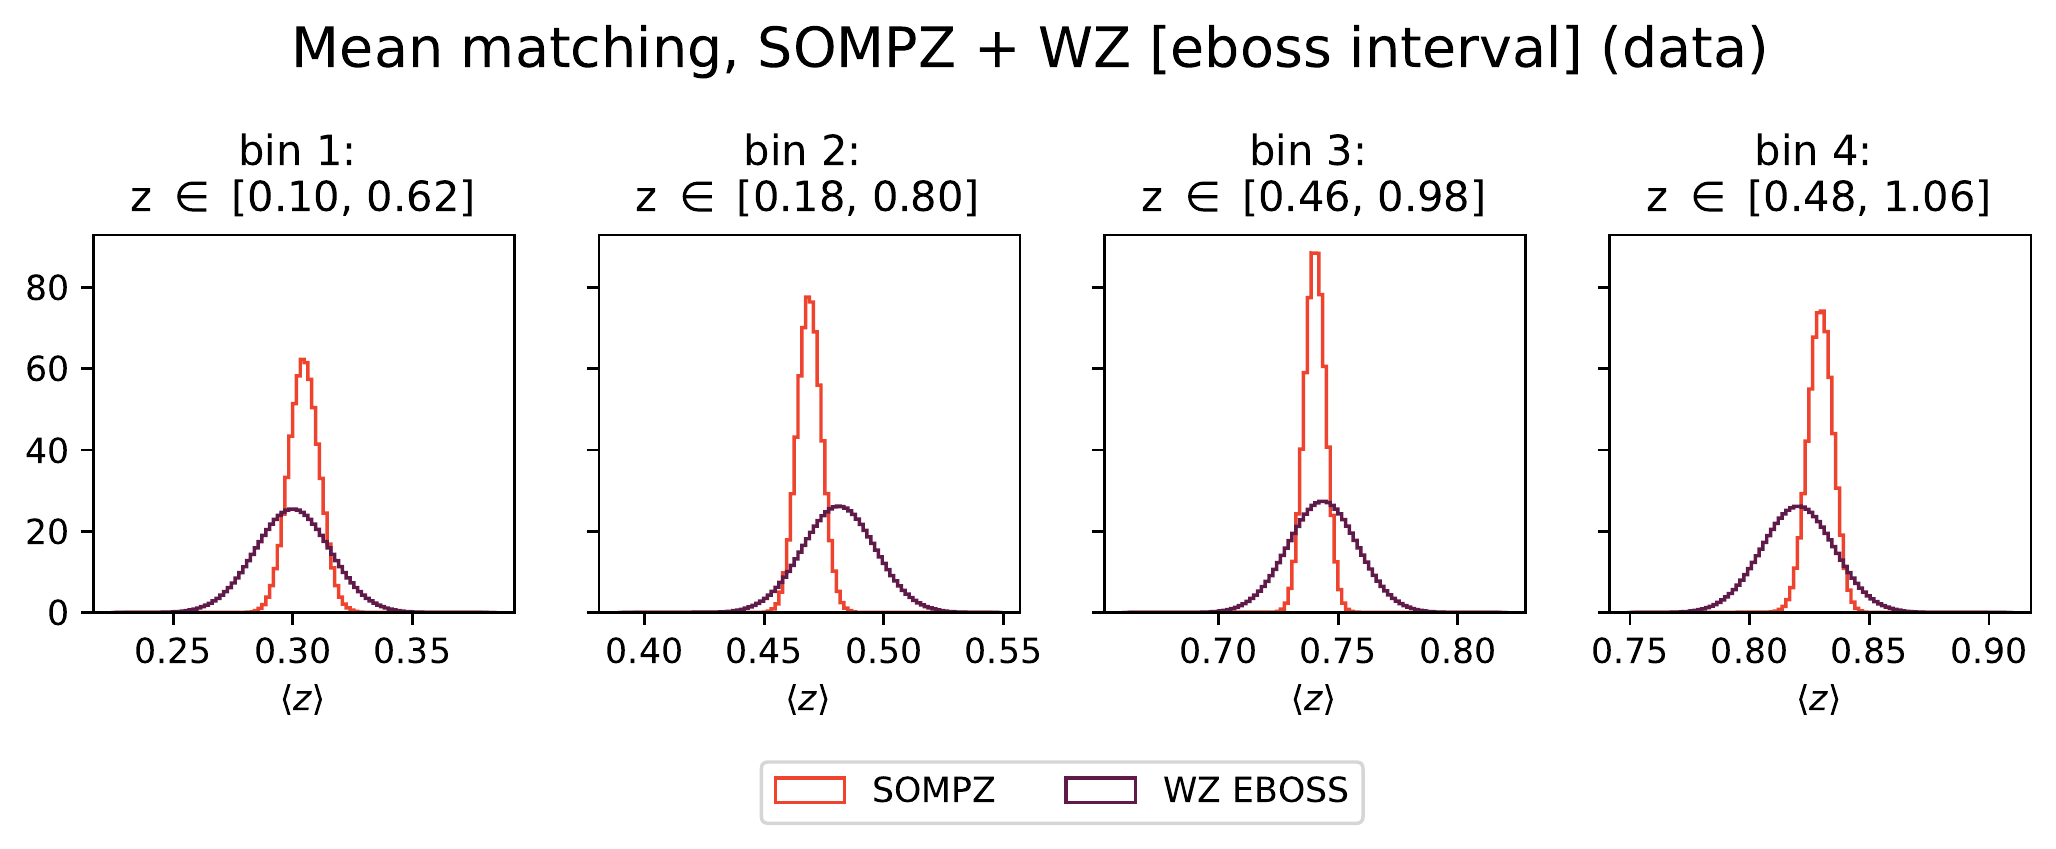}
\end{center}
\caption{Same as Fig.~\ref{fig:dz_meanmatching_SOMPZ_WZ_individual_sims}, but now on data.} 
\label{fig:dz_meanmatching_SOMPZ_WZ_individual_data}
\end{figure*}

We show in this Appendix the posteriors of the mean of the SOMPZ realisation obtained with the mean matching method when using the two reference samples individually. We show both the results obtained in simulations and in data.

In particular, Fig.~\ref{fig:dz_meanmatching_SOMPZ_WZ_individual_sims} shows the mean redshift posteriors of the SOMPZ realisations obtained in simulations. To facilitate the comparison with the clustering only prior, we computed the mean in the 2-$\sigma$ interval of the reference sample used. The first thing that can be noted is that the clustering prior is consistent - within uncertainties - with the mean of the SOMPZ realisations before combining the two pieces of information. The other thing that can be noted is that the histograms clearly show that the clustering prior is much wider than the scatter of the SOMPZ realisations, especially for the low redshift tomographic bins, which explains why the mean matching clustering likelihood does not help much tightening the posterior. Last, we note that the final scatter on the mean of the SOMPZ realisations is larger than what is shown in Fig.~\ref{fig:dz_meanmatching_SOMPZ_WZ_individual_sims}, as it gets contributions from the redshift range where there is no clustering information.

\gnote{moved this paragraph into main text, so delete?}
Fig.~\ref{fig:dz_meanmatching_SOMPZ_WZ_individual_data} shows the mean redshift posteriors of the SOMPZ realisations obtained on data, along with the WZ prior. The results are qualitatively and quantitatively very similar to what has been obtained in simulations: the clustering prior and SOMPZ realisations are consistent within errors before combining, and the mean matching clustering likelihood does not help much tightening the mean redshift posterior of the SOMPZ realisations.
